# Supplementary material for: What did Ryser Conjecture?
Source: arXiv:1801.02893 ancillary file (2018-01-09)
Supplement: Supplementary file 1 [file RyserOriginal.pdf]

# H. J. RYSER : Neuere Probleme in der Kombinatorik

## 1. Lateinische Quadrate

Sei  $n$  eine natürliche Zahl und  $S$  eine Menge von  $n$  unterschiedenen Elementen, etwa der Ziffern  $1, \dots, n$ . Unter einem lateinischen Rechteck der Ordnung  $r \times s$  ( $r, s$  natürliche Zahlen) versteht man eine  $r \times s$ -Matrix  $[a_{ij}]_{r \times s}$  aus Elementen von  $S$ , welche in keiner Zeile und in keiner Spalte Wiederholungen aufweist:

$$a_{ij} = a_{ik} \implies j = k \quad (i = 1, \dots, r),$$

$$a_{ij} = a_{kj} \implies i = k \quad (j = 1, \dots, s).$$

In jedem lateinischen Rechteck ist demnach  $r \leq n$  und  $s \leq n$ . Da es bei diesem Begriff nun weder auf die Ordnung der Ziffern noch auf die Unterscheidung von Spalten und Zeilen ankommt, kann man sich - insbesondere im Hinblick auf Satz 1.2 - auf die Betrachtung solcher lateinischer Rechtecke beschränken, bei denen  $s = n$  ist und die erste Zeile aus den Ziffern  $1, \dots, n$  in natürlicher Reihenfolge besteht:

$$a_{1j} = j \quad (j = 1 \dots n).$$

Solche lateinischen Rechtecke heißen *normalisiert*.

Ist speziell  $r = s = n$ , so spricht man von einem *lateinischen Quadrat* der Ordnung  $n$ . Ein solches heißt *normalisiert*, wenn sowohl die erste Zeile als auch die erste Spalte die Ziffern  $1, \dots, n$  in natürlicher Reihenfolge enthalten.

$$a_{1j} = j \quad (j = 1 \dots n)$$

$$a_{i1} = i \quad (i = 1 \dots n)$$

Beispiele der einfachsten normalisierten lateinischen Quadrate sind

$$[1] \quad \begin{bmatrix} 1 & 2 \\ 2 & 1 \end{bmatrix} \quad \begin{bmatrix} 1 & 2 & 3 \\ 2 & 3 & 1 \\ 3 & 1 & 2 \end{bmatrix}$$

An diese Definition knüpft sich nun die spezifische kombinatorische Frage nach der

Anzahl der verschiedenen so definierten Objekte. Offensichtlich erhält man nur ein normalisiertes lateinisches  $1 \times n$ -Rechteck. Die Anzahl der verschiedenen lateinischen  $2 \times n$ -Rechtecke ist gleich der Zahl  $D_n$  der Permutationen ohne Fixpunkte ("derangements"); diese ist leicht zu berechnen:

$$D_n = n! \cdot \left( 1 - \frac{1}{1!} + \frac{1}{2!} - \dots + (-1)^n \frac{1}{n!} \right) \approx \frac{n!}{e}$$

Ein expliziter Ausdruck für die Anzahl der lateinischen  $3 \times n$ -Rechtecke wird aber recht kompliziert, für lateinische  $4 \times n$ -Rechtecke ist die Lösung des Problems unbekannt.

Interessant ist vor allem die Frage nach der Anzahl  $l_n$  der normalisierten lateinischen Quadrate der Ordnung  $n$ . Für die Zahlen  $l_n$  ist jedoch kein expliziter Ausdruck bekannt; bis  $n = 8$  wurden sie berechnet (für  $n = 7$  von A. Sade, für  $n = 8$  von Mark Wells mit dem Computer Maniac in 8 Stunden Rechenzeit [erscheint in: J. of Combinatorial Theory]):

| $n$   | 1 | 2 | 3 | 4 | 5  | 6    | 7          | 8               |
|-------|---|---|---|---|----|------|------------|-----------------|
| $l_n$ | 1 | 1 | 1 | 1 | 56 | 9408 | 16 942 080 | 535 281 401 856 |

Es fällt auf, daß in diesen bekannten  $l_n$  für  $n \geq 4$  recht hohe Potenzen von 2 auftreten.

Anzumerken ist noch, daß die  $l_n$  als Koeffizienten einer gewissen im Zusammenhang mit Mac Mahon's "Master theorem" stehenden Potenzreihe auftreten, die jedoch zur Berechnung der  $l_n$  nicht geeignet ist.

Recht wenig ist auch sonst über lateinische Quadrate bekannt; die bekannten Resultate:

Satz 1.1. (M. Hall):

Jedes lateinische  $r \times n$ -Rechteck ( $r \leq n$ ) kann zu einem lateinischen Quadrat der Ordnung  $n$  ergänzt werden.

Beweis: Wir setzen das gegebene Rechteck als normalisiert voraus. Sei  $S_i$  die Teilmenge von  $S$ , die aus den in der  $i$ -ten Spalte nicht auftretenden Ziffern besteht ( $i = 1 \dots n$ ). Zu  $S_1, \dots, S_n$  sei  $A$  die Inzidenzmatrix, definiert durch

$$A = [a_{ik}]_{i=1, \dots, n} \quad \text{mit} \quad a_{ik} = \begin{cases} 1 & \text{falls } k \in S_i \\ 0 & \text{sonst.} \end{cases}$$

Wegen  $|S_i| = n - r$  enthält jede Zeile von  $A$  genau  $n - r$  Einsen.

Da weiter nach Definition des lateinischen Rechtecks eine beliebige Ziffer in genau  $r$  der Mengen  $S \sim S_i$  ( $i = 1 \dots n$ ) auftritt, kommt sie in genau  $n - r$  der Mengen  $S_i$  vor; und demnach enthält auch jede Spalte von  $A$  genau  $n - r$  Einsen.

Jede solche Matrix ist aber nach dem (später zitierten) Birkhoff-König-Theorem die Summe von  $n - r$  Permutationsmatrizen  $P_j$ :

$$A = P_1 + \dots + P_{n-r}$$

Setzt man nun die  $(r+i)$ -te Zeile gleich der durch  $P_i$  gegebenen Permutation der Ziffern  $(1 \dots n)$ , d.h.

$$[a_{r+i, j}] = P_i \begin{bmatrix} 1 \\ \vdots \\ n \end{bmatrix}$$

im Sinne der Matrixmultiplikation, so erhält man ein lateinisches Quadrat. Denn offensichtlich kommen in den Zeilen keine Wiederholungen vor, ebenso wenig wie in den Spalten, da die neu hinzukommenden Ziffern der Spalte  $i$  genau die Elemente von  $S_i$  sind.

Es gilt das geringfügige verallgemeinerte Resultat (hier ohne Beweis)

Satz 1.2: Ein lateinisches  $r \times s$ -Rechteck läßt sich zu einem lateinischen Quadrat der Ordnung  $n$  ergänzen genau dann, wenn

$$N(i) \geq r + s - n \quad (i = 1 \dots r),$$

wobei  $N(i)$  angibt, wievielmals  $i$  im gegebenen  $r \times s$ -Rechteck auftritt.

Das obige Resultat folgt daraus für  $s = n$ .

Das behandelte Problem kann in folgender Weise allgemeiner gestellt werden:

Sei  $S$  die aus den Ziffern  $1, \dots, n$  und dem Symbol  $x$  ("Leerstelle") bestehende Menge. Gegeben sei eine  $n \times n$ -Matrix aus Elementen von  $S$ .

Welches sind die notwendigen und hinreichenden Bedingungen dafür, daß diese Matrix durch Ersetzung von  $x$  durch Ziffern (nicht notwendig eine und dieselbe) zu einem lateinischen Quadrat ergänzt werden kann?

Oben haben wir den speziellen Fall

$$\begin{bmatrix} \text{(Ziffern)} \\ \hline x & x & . & . & . & . & . & . & . & . & x \\ . & . & . & . & . & . & . & . & . & . & . \\ . & . & . & . & . & . & . & . & . & . & . \\ x & x & . & . & . & . & . & . & . & . & x \end{bmatrix}$$

behandelt.

Im folgenden verstehen wir unter einer Reihe einer Matrix eine Zeile oder Spalte derselben.

Gegeben sei eine quadratische Matrix  $[a_{ik}]$  der Ordnung  $n$ . Eine Menge  $P = \{ (i, k) \}$  von  $n$  Index-Paaren heie ein Pfad, wenn nicht zwei ihrer Elemente zur gleichen Reihe der Matrix gehren, also wenn

$$(i, k) \in P \text{ impliziert: } (i, l) \notin P \text{ fr } l \neq k \\ \text{und } (j, k) \notin P \text{ fr } i \neq j.$$

$P$  heie Transversalpfad, wenn auerdem alle Ziffern von 1 bis  $n$  unter den  $a_{ik}$  ( $(i, k) \in P$ ) vorkommen. Z. B. ist die Hauptdiagonale einer jeden quadratischen Matrix ein Pfad, ebenso die Nebendiagonale. Die Hauptdiagonale des lateinischen Quadrates

$$\begin{bmatrix} 1 & 2 & 3 \\ 2 & 3 & 1 \\ 3 & 1 & 2 \end{bmatrix}$$

ist ein Transversalpfad, jedoch nicht seine Nebendiagonale. Das lateinische Quadrat

$$\begin{bmatrix} 1 & 2 \\ 2 & 1 \end{bmatrix}$$

hat nicht einen einzigen Transversalpfad. Das erste Beispiel scheint Spezialfall eines allgemeineren Sachverhalts zu sein; wir formulieren die folgende Vermutung:

Ein lateinisches Quadrat ungerader Ordnung hat stets einen Transversalpfad. Verifiziert wurde diese Vermutung im Fall  $n = 5$  (H. J. Ryser). Sie lt sich fr allgemeines<sup>2)</sup> leicht unter der Zusatzannahme beweisen, da es sich um ein symmetrisches lateinisches Quadrat handelt.

In diesem Fall ist die Hauptdiagonale stets ein Transversalpfad. Es gengt dazu zu zeigen, da sie eine 1 enthlt, das folgt aber daraus, da die 1 im Quadrat genau  $n$  - mal vorkommt und davon wegen der Symmetrie  $\frac{n-k}{2}$  - mal unterhalb der Hauptdiagonalen, wenn  $k$  die Zahl der Einsen auf der Hauptdiagonale ist;  $k$  kann wegen der Ungeradzahligkeit von  $n$  also nicht verschwinden.



## 2. Orthogonale Systeme lateinischer Quadrate

Seien  $A_1 = [a_{ij}^{(1)}]$ ,  $A_2 = [a_{ij}^{(2)}]$  lateinische Quadrate der Ordnung  $n \geq 3$ .

Man bilde dazu das "Überlagerungsquadrat" der geordneten Paare  $[(a_{ij}^{(1)}, a_{ij}^{(2)})]$  (Eulers "griechisch-lateinisches" Quadrat).

Sind die  $n^2$  Zahlenpaare dieses Quadrates alle verschieden, so heißen  $A_1$  und  $A_2$  orthogonal.

Z.B. sind  $\begin{bmatrix} 1 & 2 & 3 \\ 2 & 3 & 1 \\ 3 & 1 & 2 \end{bmatrix}$  und  $\begin{bmatrix} 1 & 2 & 3 \\ 3 & 1 & 2 \\ 2 & 3 & 1 \end{bmatrix}$

orthogonale lateinische Quadrate. Um zum ersteren das dazu orthogonale zweite zu finden, hat man hier die drei Transversalpfade des ersteren jeweils mit denselben Ziffern besetzt.

Eine Menge von lateinischen Quadraten heißt orthogonales System von lateinischen Quadraten, wenn ihre Elemente paarweise orthogonal sind.

Es kann nicht zu große orthogonale Systeme geben, das zeigt der

Satz 2. Für jedes orthogonale System  $A_1, \dots, A_t$  ( $A_\tau = [a_{ij}^{(\tau)}]$ ,  $\tau = 1, \dots, t$ ) von  $t$  lateinischen Quadraten der Ordnung  $n$  ( $t \geq 2$ ,  $n \geq 3$ ) gilt

$$t \leq n - 1.$$

Beweis: Offensichtlich ändert eine Umbenennung der Matrixelemente nichts an der Orthogonalität von Quadraten, und so können wir annehmen, daß  $A_1 \dots A_t$  die gleiche erste Zeile haben, bestehend aus den Ziffern  $1 \dots n$  in natürlicher Reihenfolge. Die  $a_{21}^{(\tau)}$  ( $\tau = 1, \dots, t$ ) müssen nun alle verschieden sein, ferner dürfen sie den Wert 1 nicht annehmen. Daraus folgt der Satz.

Ist  $t = n - 1$ , so spricht man von einem vollständigen System orthogonaler lateinischer Quadrate.

Es erhebt sich daher die Frage, für welche  $n$  denn vollständige orthogonale Systeme von Quadraten der Ordnung  $n$  existieren.

Satz 2. Für  $n = p^a \geq 3$  ( $p$  prim) existiert ein vollständiges System von orthogonalen lateinischen Quadraten der Ordnung  $n$ .  
(bewiesen von Veblen und Bassey)

Beweis: Sei  $S = GF(p^a) = \{a_0 = 0, a_1 = 1, a_2, \dots, a_{n-1}\}$ .

Durch die Festsetzung

$$A_e = [a_{ij}^{(e)}] \text{ mit } a_{ij}^{(e)} = a_e a_i + a_j \\ (i, j = 0, \dots, n-1; e = 1, \dots, n-1)$$

ist ein vollständiges System von orthogonalen Quadraten definiert. Zunächst vermuteten wir, daß  $A_e$  lateinische Quadrate sind:

- gleiche Elemente in einer Zeile würde bedeuten

$$a_e a_i + a_j = a_e a_{i'} + a_j,$$

woraus  $a_j = a_{j'}$  und also  $j = j'$  folgen würde;

- gleiche Elemente in einer Spalte hieße

$$a_e a_i + a_j = a_e a_{i'} + a_j,$$

also  $a_i = a_{i'}$  und  $i = i'$ .

#### Nachweis der Orthogonalität

Wir haben die Annahme

$$(a_{ij}^{(e)}, a_{ij'}^{(f)}) = (a_{i'j}^{(e)}, a_{i'j'}^{(f)})$$

mit  $e \neq f$  und  $(i, j) \neq (i', j')$  zu widerlegen. Aus ihr würde folgen

$$a_e a_i + a_j = a_e a_{i'} + a_{j'},$$

$$\text{und } a_f a_i + a_j = a_f a_{i'} + a_{j'},$$

Subtraktion beider Gleichungen ergäbe

$$a_i (a_e - a_f) = (a_e - a_f) a_{i'}, \quad \text{also } a_i = a_{i'},$$

und folglich auch  $a_j = a_{j'}$ , im Widerspruch zur Annahme.

Eine schwierige Frage ist die der Eindeutigkeit von vollständigen orthogonalen Systemen. Eindeutigkeit konnte nachgewiesen werden bis zur Ordnung 8; für  $n = 9$  ist sie verletzt.

Dagegen ist über die Existenz orthogonaler (i. a. nicht vollständiger) Systeme Genaueres bekannt:

Satz 2.3 (Mac Neish)

Sei  $n = p_1^{\alpha_1} \dots p_N^{\alpha_N}$  ( $p_i$  prim),  $t = \min_{i=1 \dots N} (p_i^{\alpha_i} - 1) \geq 2$ .

Dann existieren  $t$  paarweise orthogonale lateinische Quadrate der Ordnung  $n$ .

Dem Beweis dieses Satzes schicken wir zwei Lemmata voraus:

Lemma 2.1:

Einem System von  $t$  orthogonalen lateinischen Quadraten  $A_1, \dots, A_t$  entspricht eineindeutig das folgende Schema

|     |     |                |                |     |   |   |
|-----|-----|----------------|----------------|-----|---|---|
| 1   | 1   | 1. Zeile $A_1$ | 1. Zeile $A_2$ | ... | } | n |
| 1   | 2   |                |                |     |   |   |
| ... | ... |                |                |     |   |   |
| 1   | n   |                |                |     |   |   |
| 2   | 1   | 2. Zeile $A_1$ | 2. Zeile $A_2$ | ... | } | n |
| 2   | 2   |                |                |     |   |   |
| ... | ... |                |                |     |   |   |
| 2   | n   |                |                |     |   |   |
| ... | ... | ...            | ...            | ... |   |   |
| n   | 1   | n. Zeile $A_1$ | n. Zeile $A_2$ | ... | } | n |
| n   | 2   |                |                |     |   |   |
| ... | ... |                |                |     |   |   |
| n   | n   |                |                |     |   |   |

welches die Eigenschaft hat, daß jede  $n^2 \times 2$  - Untermatrix alle  $n^2$  aus den Ziffern  $1, \dots, n$  gebildeten Paare enthält.

Beweis: Die  $A_\tau$  ( $\tau = 1, \dots, t$ ), wie angegeben aus dem Schema abgeleitet, bilden ein System von orthogonalen lateinischen Quadraten: lateinisch, weil aus der Gestalt der 1. bzw. 2. Spalte des Schemas folgt, daß in einer Zeile bzw. Spalte von  $A_\tau$  nicht zwei identische Ziffern vorkommen können; orthogonal, weil die Elemente von  $A_\tau$  und  $A_{\tau'} (\tau \neq \tau')$  im Schema eine  $n^2 \times 2$  - Matrix bilden und somit nach Voraussetzung alle  $A_\tau - A_{\tau'}$  - Paare verschieden sind. Diese Überlegung zeigt zugleich auch, daß ein System von  $t$  orthogonalen lateinischen Quadraten, auf die angegebene Weise zu einem  $n^2 \times (t+2)$ -Schema zusammengefaßt, die fragliche Eigenschaft hat.

Lemma 2.2: Wenn es  $t$  orthogonale lateinische Quadrate der Ordnung  $n$  und  $t$  von der Ordnung  $n'$  gibt, dann gibt es auch  $t$  orthogonale lateinische Quadrate von der Ordnung  $n \cdot n'$ .

Beweis: Nach Lemma 2.1 brauchen wir nur die zugehörigen  $n^2 \times (t+2)$  - bzw.  $n'^2 \times (t+2)$  - Schemata  $B = (b_{ij})$  bzw.  $B' = (b'_{kl})$  zu betrachten. Aus ihnen bilden wir ein  $(n \cdot n')^2 \times (t+2)$  - Schema  $B^*$  durch die Festsetzung

$$b^*_{(i,i'), j} = (b_{ij}, b'_{i'j}) \text{ mit } \begin{cases} (i, i') = (1, 1), \dots, (n, n'), \\ j = 1, \dots, t+2 \end{cases}$$

wonach die Elemente dieses neuen Schemas nun die aus den Ziffern  $1, \dots, n$  und  $1, \dots, n'$  gebildeten Paare sind.

Das neue Schema hat ebenfalls die Eigenschaft, daß jede  $(n \cdot n')^2 \times 2$  - Untermatrix alle  $(n \cdot n')^2$  aus  $(1, 1), \dots, (n, n')$  gebildeten Paare enthält.

Aus Lemma 2.1 folgt die Behauptung.

Der Satz folgt nun durch Anwendung des vorhergehenden Satzes und mehrfache Anwendung von Lemma 2.2.

Satz 2.3. sagt nichts aus im Fall  $n = 2$  u mit ungeradem  $u$ ; in allen anderen Fällen liefert er die Existenz von mindestens zwei orthogonalen lateinischen Quadraten.

Euler vermutete sogar, daß in diesem Fall ( $n \equiv 2 \pmod{4}$ ) kein Paar von orthogonalen lateinischen Quadraten existiert. Diese Vermutung ist trivialerweise richtig für  $n = 2$  und konnte auch für den nächstschwierigen Fall  $n = 6$  überprüft und verifiziert werden (Tarry, 1900). Um so erstaunlicher ist das Ergebnis von Bose, Shrikhande und Parker (1960), welches sagt, daß diese Fälle die einzigen sind, in welchen Euler's Vermutung stimmt:

Satz 2.4. Es gibt Paare orthogonaler lateinischer Quadrate von jeder Ordnung  $n \neq 2$  und  $\neq 6$ .

Den Beweis geben wir wegen seiner Kompliziertheit hier nicht wieder, eine Widerlegung der Eulerschen Vermutung enthält aber schon der elegantere Beweis für den Fall  $n \equiv 10 \pmod{12}$  (siehe [1]).



### 3. Projektive Ebenen

Sei  $n \geq 3$ . Vom Standpunkt der Kombinatorik kann man projektive Ebenen wie folgt einführen:

Definition: Eine projektive Ebene der Ordnung  $n$  ist gegeben durch ein vollständiges System orthogonaler lateinischer Quadrate der Ordnung  $n$ .

Äquivalent dazu ist die Angabe einer quadratischen Null-Eins-Matrix  $A$  der Ordnung  $m = n^2 + n + 1$  mit  $AA^T = nI + J$ , wobei

$$I = (\delta_{ij})_{m \times m} \quad \text{und} \quad J = (1)_{m \times m}.$$

Denn sei ein vollständiges System orthogonaler lateinischer Quadrate der Ordnung  $n$  gegeben; man ordne ihnen gemäß Lemma 2.1 ein  $n^2 \times (n+1)$ -Schema zu. Die Zeilen dieses Schemas seien  $Z_1, \dots, Z_{n^2}$ . Ferner nehme man die folgenden (paarweise verschiedenen) Symbole  $Z_{n^2+1}, \dots, Z_{n^2+n+1}$  hinzu,

und bezeichne mit  $G_{ij}$  ( $i = 1 \dots n; j = 1 \dots n+1$ ) die Menge aller  $Z_k$  mit  $i$  in der  $j$ -ten Spalte, vereinigt mit  $Z_{n^2+j}$ . Nach Voraussetzung sind alle  $G_{ij}$  verschieden.

Schließlich bezeichne  $G$  die Menge der Symbole  $Z_{n^2+1}, \dots, Z_{n^2+n+1}$ .

$A$  sei nun die  $(n^2 + n + 1) \times (n^2 + n + 1)$ -Inzidenzmatrix der  $Z_k$  bezüglich der  $G$ 's. Dann ist klar, daß jedes  $G$  genau  $n+1$   $Z$ 's enthält, und jedes  $Z$  in genau  $n+1$   $G$ 's enthalten ist, woraus die Matrixgleichung für  $A$  folgt.

In geometrischer Sprache gesprochen, sind die  $Z$ 's die Punkte und die  $G$ 's Geraden.

Sei umgekehrt  $A$  mit den genannten Eigenschaften gegeben. Wir fassen  $A$  als Inzidenzmatrix von  $n^2 + n + 1$  "Punkten"  $Z_j$  und ebensovielen "Geraden"  $G_k$  auf.

Eine Gerade,  $G_1$  etwa, werde festgehalten, auf ihr mögen die Punkte  $P_1, \dots, P_{n+1}$  liegen.  $Q_1, \dots, Q_n$  seien die Punkte, die nicht auf  $G_1$  liegen.

Wie aus der Matrixgleichung folgt, verlaufen durch jeden Punkt genau  $n+1$  Geraden. Die  $n$  Geraden durch  $P_j$ , verschieden von  $G_1$ , mögen mit den Ziffern  $1, \dots, n$  belegt werden, und zwar für jedes  $j$ . Damit tragen alle Geraden bis auf  $G_1$  eine Nummer  $s \in \{1, \dots, n\}$ .

Sei  $C = [C_{ij}] = [\text{Nummer von } \overline{Q_i P_j}]$ . Durch zwei Punkte verläuft ja genau eine Gerade, wie aus der Matrixgleichung direkt folgt. Es ist nun leicht nachzuprüfen, daß  $C$  ein Schema von der in Lemma 2.1. beschriebenen Gestalt ist. Aus ihm lassen sich  $n - 1$  paarweise orthogonale lateinische Quadrate ableiten.

Das kombinatorische Problem, daß sich an diese Betrachtung knüpft, ist die Bestimmung derjenigen  $n$ , für welche projektive Ebenen der Ordnung  $n$  existieren. Für  $n = p^\alpha$  mit  $p$  prim folgt die Existenz einer projektiven Ebene dieser Ordnung aus Satz 2.2. Das kleinste  $n$ , für welches dieses Problem ungelöst ist, ist  $n = 10$ . Hier hat man noch nicht einmal drei paarweise orthogonale Quadrate finden können (trotz Parker's umfangreicher Computer-Rechnungen). Parker erhielt durch unsystematisches Suchen 84 lateinische Quadrate der Ordnung 10. Darunter hatten 33 keinen orthogonalen "Partner", 29 hatten genau einen, 15 zwei, 2 drei, 3 vier und 2 hatten fünf orthogonale Partner.

Es zeigt sich, daß ca. 50% aller zufällig gefundenen Quadrate orthogonale Partner haben.

Wir geben noch eine Idee an, die in diesem Zusammenhang nützlich ist. In dem lateinischen Quadrat

$$\begin{bmatrix} 1 & 2 & 3 \\ 2 & 3 & 1 \\ 3 & 1 & 2 \end{bmatrix}$$

findet man drei Transversalpfade, die sinnfällig durch die drei Matrizen

$$\begin{bmatrix} 1 & 0 & 0 \\ 0 & 1 & 0 \\ 0 & 0 & 1 \end{bmatrix}, \begin{bmatrix} 0 & 1 & 0 \\ 0 & 0 & 1 \\ 1 & 0 & 0 \end{bmatrix}, \begin{bmatrix} 0 & 0 & 1 \\ 1 & 0 & 0 \\ 0 & 1 & 0 \end{bmatrix}$$

gekennzeichnet werden, welche sich zu  $J = (1)_{3 \times 3}$  aufaddieren:

die Transversalpfade sind paarweise "disjunkt".

Besetzt man den ersten Transversalpfad mit Einsen, den zweiten mit Zweien u. s. f., so erhält man offenbar einen zu dem gegebenen Quadrat orthogonalen Partner.

Es gilt sogar ganz allgemein:

Genau dann hat ein lateinisches Quadrat der Ordnung  $n$  einen orthogonalen Partner, wenn es  $n$  paarweise disjunkte Transversalpfade hat.

Beispiel:

|   |   |   |   |   |   |   |   |   |   |
|---|---|---|---|---|---|---|---|---|---|
| 5 | 1 | 7 | 3 | 4 | 0 | 6 | 2 | 8 | 9 |
| 1 | 2 | 3 | 4 | 5 | 6 | 7 | 8 | 9 | 0 |
| 7 | 3 | 4 | 5 | 6 | 2 | 8 | 9 | 0 | 1 |
| 3 | 4 | 5 | 6 | 7 | 8 | 9 | 0 | 1 | 2 |
| 4 | 5 | 6 | 7 | 8 | 9 | 0 | 1 | 2 | 3 |
| 0 | 6 | 2 | 8 | 9 | 5 | 1 | 7 | 3 | 4 |
| 6 | 7 | 8 | 9 | 0 | 1 | 2 | 3 | 4 | 5 |
| 2 | 8 | 9 | 0 | 1 | 7 | 3 | 4 | 5 | 6 |
| 8 | 9 | 0 | 1 | 2 | 3 | 4 | 5 | 6 | 7 |
| 9 | 0 | 1 | 2 | 3 | 4 | 5 | 6 | 7 | 8 |

ist ein lateinisches Quadrat der Ordnung 10 (angegeben von Parker). Vertauscht man an den eingerahmten Stellen 0 und 5 sowie 2 und 7, so erhält man ein zyklisches lateinisches Quadrat (gerader Ordnung), welches - wie man leicht nachprüft - keinen Transversalpfad besitzen kann und folglich auch keinen orthogonalen Partner hat. Dagegen hat aber das angegebene Quadrat 5504 Transversalpfade und approximativ  $10^6$  orthogonale Partner.

Die obige Darstellung lateinischer Quadrate mittels  $n$  Null-Eins-Matrizen, welche die Lage der Transversalpfade angeben, kann noch verfeinert werden. Man bilde zu gegebenem lateinischem Quadrat  $[a_{ij}]_{n \times n}$  die  $n$  Matrizen

$$[d_{ijk}] \text{ mit } d_{ijk} = \begin{cases} 1 & \text{für } a_{ij} = k \\ 0 & \text{sonst} \end{cases}.$$

Diese bilden einen sogenannten lateinischen Würfel, eine dreidimensionale Null-Eins-Matrix, die in jeder (achsenparallelen) Reihe genau eine 1 besitzt. Genau wenn dies Ausgangsquadrat einen orthogonalen Partner hat, existiert eine König-Birkhoff-Zerlegung des zugeordneten Würfels in  $n$  Würfel mit genau einer 1 in jeder achsenparallelen Ebene. (siehe Artikel von Ryser und Jurkat; erscheint im J. of Algebra).



4. Zwei kombinatorische Schlußweisen bei Null - Eins - Matrizen

An Hand der folgenden beiden Probleme sollen zwei charakteristische Schlußweisen der Kombinatorik vorgeführt werden.

Problem 1: Sei  $A = (a_{ij})$  eine Null-Eins-Matrix der Ordnung  $m \times n$  derart, daß jedes Element von  $A$  positiv ist und  $A$  (nach eventueller Permutation von Zeilen und Spalten) keine Untermatrix der Gestalt

$$\begin{bmatrix} 0 & 1 & 1 \\ 1 & 0 & 1 \\ 1 & 1 & 0 \end{bmatrix}$$

besitzt.

Man zeige, daß  $A$  eine Zeile aus lauter Einsen besitzt.

Problem 2: Sei  $A$  eine symmetrische Null-Eins-Matrix der Ordnung  $v$ , derart daß

$$AA^T = (k-\lambda)I + \lambda J,$$

$$\text{wo } I = (\delta_{ij})_{v \times v}, J = (1)_{v \times v}$$

$$\text{und } 0 < \lambda < k < v-1.$$

Zeige, daß  $A$  unter der Annahme,  $k-\lambda$  sei kein Quadrat, genau  $k$  Einsen in seiner Hauptdiagonale hat.

(Dieses Problem tritt im Zusammenhang mit  $(b, k, \lambda)$  - Konfigurationen auf, siehe [1]).

Lösung von Problem 1:

Wir führen den Beweis durch Induktion über die Zahl der Spalten. Für  $n=1$  und  $n=2$  ist die Behauptung wahr. Sei also  $n \geq 3$ .

Es bezeichne  $B$  die Matrix, welche durch Weglassen der ersten Spalte aus  $A$  entsteht. Offensichtlich ist dann  $B^T B$  eine Untermatrix von  $A^T A$  und hat somit nur positive Elemente. Damit gilt nach Induktionsvoraussetzung, daß  $B$  eine Zeile aus lauter Einsen besitzt; das sei o. B. d. A. die erste Zeile von  $B$ .

Ist nun  $a_{11} = 1$ , so ist der Satz bewiesen; wir betrachten daher nur den ungünstigen Fall  $a_{11} = 0$ .

Wiederholen wir die eben angewandte Schlußweise, indem wir nur die 2. statt der ersten Spalte von  $A$  weglassen (und gegebenenfalls die letzten  $m-1$  Zeilen permutieren), und tun dann dasselbe noch für die 3. Spalte, (wobei wir stets die



ungünstigen Fälle annehmen), so erhalten wir, daß A die folgende Gestalt hat (bis auf Permutation von Zeilen und Spalten):

$$\begin{bmatrix} 0 & 1 & 1 & 1 & \dots & 1 \\ 1 & 0 & 1 & 1 & \dots & 1 \\ 1 & 1 & 0 & 1 & \dots & 1 \\ \vdots & \vdots & \vdots & \vdots & \ddots & \vdots \end{bmatrix}$$

Diese Matrix besitzt eine Untermatrix der verbotenen Form, und folglich konnte der für uns ungünstige Fall nicht stets eintreten.

#### Lösung von Problem 2:

Wir untersuchen das Spektrum  $\{\lambda_1, \dots, \lambda_v\}$  von A.

Aus der Matrixgleichung folgt, daß A genau k Einsen in jeder Zeile hat; daher ist  $\lambda_1 = k$  ein Eigenwert von A (mit dem Eigenvektor  $\begin{pmatrix} 1 \\ 1 \end{pmatrix}$ ).

Wegen  $AA^T = A^2$  hat  $(k - \lambda) I + \lambda J$  die Eigenwerte  $\lambda_1^2, \lambda_2^2, \dots, \lambda_v^2$ . Nun hat J aber als einzigen von 0 verschiedenen Eigenwert v, da es Rang 1 hat. Daher sind die übrigen Eigenwerte von  $AA^T$  alle  $= k - \lambda$ . D. h. das Spektrum von A ist  $= \{k, \sqrt{k-\lambda}, -\sqrt{k-\lambda}\}$ .

Und daher gilt für die Spur

$$\text{Spur } A = k + a\sqrt{k-\lambda} - b\sqrt{k-\lambda} \text{ mit } a, b \text{ ganz.}$$

Da aber Spur A ganzzahlig sein muß und  $k - \lambda$  kein Quadrat ist, gilt  $a = b$ .

Die Spur von A ist damit  $= k$ .

## 5. Der Heiratssatz

Wir beweisen in diesem Paragraphen zwei verwandte Sätze.

Satz 5.1. (König-Egerváry):

Sei A eine Null-Eins-Matrix der Ordnung  $m \times n$ . Die Minimalanzahl der Reihen, welche sämtliche Einsen von A enthalten, ist gleich der Maximalanzahl der Einsen, von denen je zwei nicht auf einer Reihe liegen.

Beispiel:

$$\rightarrow \begin{array}{c} \downarrow \quad \downarrow \\ \begin{bmatrix} 1 & 0 & \underline{1} & 1 \\ 0 & \underline{1} & 0 & 0 \\ \underline{1} & 0 & 0 & 0 \\ 1 & 0 & 0 & 0 \end{bmatrix} \end{array}$$

Beweis: Sei  $r$  die Minimalzahl der Reihen von  $A$ , welche alle Einsen von  $A$  enthalten, und sei  $e$  die Maximalzahl der Einsen, von denen nicht zwei auf einer Reihe liegen.

Es ist  $r \geq e$ , da keine der  $r$  Reihen eines Minimalsystems von Reihen zwei Einsen eines Maximalsystems von Einsen enthält. Zu zeigen bleibt  $r \leq e$ .

Wir fixieren dazu ein Minimalsystem von Reihen, das etwa aus  $z$  Zeilen und  $s$  Spalten bestehe (also  $z + s = r$ ). O. B. d. A. seien diese  $z$  Zeilen und  $s$  Spalten die ersten  $z$  Zeilen und  $s$  Spalten der Matrix:

$$A = \begin{bmatrix} A_{11} & A_{12} \\ \underbrace{A_{21}}_s & 0 \end{bmatrix} \begin{matrix} \} z \\ \end{matrix},$$

wo  $A_{11}$  eine  $z \times s$ -Matrix ist. Sei zunächst  $0 < z < m$ .

Nun hat  $A_{12}$  ein Maximalsystem von  $z$  Einsen; denn sonst wäre - für  $A_{12}$  kann man den Satz als bewiesen annehmen - auch die Mächtigkeit eines Minimalsystems von Reihen von  $A_{12}$  kleiner als  $z$ , was zusammen mit den  $s$  ersten Spalten von  $A$  ein System von weniger als  $r$  überdeckenden Reihen von  $A$  ergäbe, im Widerspruch zur Minimalität von  $r$ . Ebenso erhält man ein Maximalsystem von  $s$  Einsen in  $A_{21}$ . Insgesamt haben wir also in  $A$  ein Maximalsystem von mindestens  $s + z = r$  Einsen, d. h.  $e \geq r$ . In den Fällen  $z = m$  bzw.  $z = 0$  kann man  $A$  bzw.  $A^T$  als Inzidenzmatrix eines Systems von  $n$  bzw.  $m$  Mengen betrachten, für welche die Behauptung eine Konsequenz des folgenden Satzes ist.

Nun soll uns der Heiratssatz von P. Hall beschäftigen: Zunächst eine

Definition: Seien  $S_1, \dots, S_m$  Teilmengen von  $S$ .

Ein  $m$ -tupel  $[a_1, \dots, a_m]$  verschiedener Elemente von  $S$  mit  $a_i \in S_i$  ( $i=1, \dots, m$ ) heißt ein individuelles Vertretersystem.

Der Heiratssatz gibt eine notwendige und hinreichende Bedingung dafür, daß ein System  $S_1, \dots, S_m$  von Teilmengen ein individuelles Vertretersystem besitzt.

Satz 5.2  $S_1, \dots, S_m$  haben ein individuelles Vertretersystem genau dann, wenn  
 $|S_{i_1} \cup \dots \cup S_{i_k}| \geq k$  für alle  $k = 1 \dots m$  und alle  $k$ -elementigen  
Teilmengen  $\{i_1, \dots, i_k\}$  von  $\{1, \dots, m\}$ .

Beweis: Es ist nur nötig, die Hinlänglichkeit der Bedingung zu beweisen. Für  $m=1$  ist sie trivial. Um sie auch für  $m$  nachzuweisen, wenn sie für alle  $m' < m$  richtig ist, machen wir die folgende Fallunterscheidung.

Fall 1: Für alle  $k = 1, \dots, m-1$  und alle  $k$ -elementigen Teilmengen  $\{i_1, \dots, i_k\}$  von  $\{1, \dots, m\}$  ist  $|S_{i_1} \cup \dots \cup S_{i_k}| \geq k+1$ .

Fall 2: Für ein  $k \in \{1, \dots, m-1\}$  existiert eine  $k$ -elementige Teilmenge  $\{i_1, \dots, i_k\}$  von  $\{1, \dots, m\}$  mit  $|S_{i_1} \cup \dots \cup S_{i_k}| = k$ .

Im ersten Fall fixiere man ein  $a_1 \in S_1$  und setze

$$S'_j = S_j - \{a_1\} \quad (j = 2, \dots, m).$$

Dieses Mengensystem erfüllt dann die Bedingung des Satzes und hat somit nach Induktionsvoraussetzung ein individuelles Vertretersystem  $(a_2, \dots, a_m) = (a_1, \dots, a_m)$  ist dann ein individuelles Vertretersystem für  $S_1, \dots, S_m$ .

Im zweiten Fall seien die Ausnahmeindizes etwa  $\{i_1, \dots, i_k\} = \{1, \dots, k\}$ .

Nach Induktionsvoraussetzung haben dann  $S_1, \dots, S_k$  ein individuelles Vertretersystem  $(a_1, \dots, a_k)$ . Nun erfüllen die

$$S_j^* := S_j - \{a_1, \dots, a_k\} \quad (j = k+1, \dots, m)$$

die Bedingung des Satzes und besitzen somit ein individuelles Vertretersystem  $(a_{k+1}, \dots, a_m)$ ; denn wenn etwa

$$|S_{k+1}^* \cup \dots \cup S_{k+k^*}^*| < k^*$$

wäre, so wäre auch

$$|S_1 \cup \dots \cup S_k \cup S_{k+1} \cup \dots \cup S_{k+k^*}| < k + k^*$$

im Widerspruch zur Voraussetzung.

$(a_1, \dots, a_m)$  ist ein individuelles Vertretersystem von  $S_1, \dots, S_m$ .

Damit ist der Beweis von Satz 5.2. beendet; eine schärfere Aussage wird in [1] bewiesen.



## 6. Permanenzen

Sei  $A = [a_{ij}]$  eine  $m \times n$  - Matrix ( $m \leq n$ ). Die Permanente von  $A$  ist definiert durch

$$\text{per } A = \sum_{\substack{\text{alle Permutationen} \\ \{i_1, \dots, i_m\} \text{ von} \\ \{1, \dots, m\}}} a_{1i_1} \cdots a_{mi_m}.$$

Der Zusammenhang mit den individuellen Vertretersystemen ist der folgende: Seien  $S_1, \dots, S_m$  Teilmengen einer  $n$ -elementigen Menge  $S$  mit  $m \leq n$ , und sei  $A$  die Inzidenzmatrix dieses Systems. Die Anzahl aller individuellen Vertretersysteme ist  $\text{per } A$ .

Die Permanente einer Matrix ist oft sehr schwierig zu berechnen. Die folgende Formel, die wir ohne Beweis aus [1] zitieren, reduziert die Rechnungen ein wenig bei  $n \times n$  - Matrizen:

$$\text{per } A = S(A) - \sum_{A_1} S(A_1) + \sum_{A_2} S(A_2) - \dots + (-1)^{n-1} \sum_{A_{n-1}} S(A_{n-1}), \quad (6.1)$$

wo  $A_r$  eine  $n \times (n-r)$  Untermatrix von  $A$  bezeichnet und  $S(A_r)$  das Produkt über alle Zeilensummen von  $A_r$  ist.

Wenn wir nach dieser Formel z. B. die Permanente von  $J-I$  berechnen, erhalten wir den folgenden Ausdruck:

$$\text{per } (J-I) = \sum_{r=0}^{n-1} (-1)^r \binom{n}{r} (n-r)^r (n-r-1)^r.$$

Andererseits ist natürlich  $\text{per } (J-I)$  gleich der Versetzungszahl  $D_n$  ("derangement number") von  $n$  Objekten, also  $= n! \left(1 - \frac{1}{1!} + \dots + (-1)^n \frac{1}{n!}\right)$ , wonach also

$$n! \left(1 - \frac{1}{1!} + \dots + (-1)^n \frac{1}{n!}\right) = \sum_{r=0}^{n-1} (-1)^r \binom{n}{r} (n-r)^r (n-r-1)^r.$$

$$X = \begin{bmatrix} x & y & 0 \\ 0 & 0 & y \\ y & 0 & x \end{bmatrix} \quad n \times n$$

in zwei verschiedenen Weisen berechnet.

Einerseits ist natürlich  $\text{per } X = x^n + y^n$ . Andererseits ergibt die Anwendung von (6.1)

$$\begin{aligned} \text{per } X &= \sum_{r=0}^{n-1} (-1)^r S(X_r) \\ &= \sum_{r=0}^{n-1} (-1)^r a_r (xy)^r (x+y)^{n-2r}, \end{aligned}$$

wobei  $a_r$  die Zahl der Möglichkeiten ist, aus einem Kreis von  $n$  Objekten  $r$  nicht benachbarte auszuwählen.

Es gilt nach einem Lemma von Kaplanski (s. [1] S. 34) :

$$a_r = \frac{n}{n-r} \binom{n-r}{r} \quad (\text{offensichtlich} = 0 \text{ für } r > \left\lfloor \frac{n}{2} \right\rfloor).$$

Damit haben wir

$$x^n + y^n = \sum_{r=0}^{\left\lfloor \frac{n}{2} \right\rfloor} (-1)^r \frac{n}{n-r} \binom{n-r}{r} (xy)^r (x+y)^{n-2r}.$$

Ähnlich wie im Fall von Determinanten interessiert hier die Frage, für welche Matrizen  $A$   $\text{per } A \neq 0$  ist.

Eine quadratische Matrix der Ordnung  $n$  heißt **doppelt stochastisch**, wenn ihre Elemente nichtnegativ sind und sämtliche Zeilen- und Spaltensummen gleich 1 sind.

Für doppelt stochastische Matrizen  $A$  ist  $\text{per } A$  stets positiv. Das folgt unmittelbar aus dem Birkhoff-König-Theorem:

Satz 6.1. Sei  $A$  doppelt stochastisch von der Ordnung  $n$ . Dann ist  $A = c_1 P_1 + \dots + c_t P_t$ , wobei die  $P_i$  Permutationsmatrizen und  $c_1, \dots, c_t$  nichtnegative reelle Zahlen mit  $\sum c_i = 1$  sind.

Beweis:  $A$  hat  $n$  positive Elemente, die paarweise verschiedenen Reihen angehören; denn andernfalls könnte man die positiven Elemente von  $A$  nach Satz 5.1. mit  $z$  Zeilen und  $s$  Spalten überdecken, wo  $z + s < n$ ; aber dann wäre  $A$  nicht doppelt stochastisch. Nun sei  $P_1$  die Permutationsmatrix, die genau an den entsprechenden Stellen Einsen hat; sei  $c_1$  das kleinste der ausgewählten  $n$  positiven Elemente. Dann ist  $A - c_1 P_1$  eine Matrix aus nichtnegativen Elementen, deren Zeilen- und Spaltensummen alle gleich  $1 - c_1$  sind.

Wiederholte Anwendung der vorangehenden Schlußweise auf  $A - c_1 P_1$  statt auf  $A$  usw. ergibt schließlich die gewünschte Darstellung.

Anmerkung: Ist speziell  $A$  eine Null-Eins-Matrix, mit identischen Zeilen- und Spaltensummen, so findet man auf diese Weise natürlich eine Darstellung mit  $c_i = 1$  für alle  $i$ .

Eine scharfe untere Abschätzung von  $\text{per } A$  für doppelt stochastische Matrizen  $A$  ist noch nicht bekannt. Nur für kleine Werte von  $n$  ( $n \leq 4$ ) konnte die Vermutung von van der Waerden verifiziert werden, welche besagt, daß

$$\text{per } A \geq \frac{n!}{n^n}$$

gilt, mit Gleichheit, genau wenn  $A = \frac{1}{n} J$ .

Wir überprüfen sie kurz für  $n = 2$ : offensichtlich hat eine zweireihige doppelt stochastische Matrix die Gestalt

$$\begin{bmatrix} x & 1-x \\ 1-x & x \end{bmatrix}$$

mit  $0 \leq x \leq 1$ , und daher ist

$$\text{per} \begin{bmatrix} x & 1-x \\ 1-x & x \end{bmatrix} = x^2 + (1-x)^2 \geq \frac{1}{2} = \frac{2!}{2^2}$$

Marcus und Mine (in: Permanents, Am. Math. Monthly 72, (1965), 577-591) konnten das schwächere Resultat beweisen:

Satz 6.2. Zu einer doppelt stochastischen Matrix  $A = [a_{ij}]$  existiert eine Permutation  $\sigma$  der Ziffern  $\{1, \dots, n\}$  derart, daß

$$\prod_{j=1}^n a_j \leq (j) \leq \frac{1}{n^n}.$$

Man könnte auf den Gedanken kommen, die van der Waerden'sche Vermutung durch die folgende zu verallgemeinern:

$$\text{per}(AB) \leq \min(\text{per } A, \text{per } B).$$

Diese Ungleichung wurde jedoch von Jurkat durch das Gegenbeispiel

$$A = \frac{1}{24} \begin{bmatrix} 11 & 5 & 8 \\ 13 & 11 & 0 \\ 0 & 8 & 16 \end{bmatrix},$$

$$B = \frac{1}{2} \begin{bmatrix} 1 & 1 & 0 \\ 1 & 1 & 0 \\ 0 & 0 & 2 \end{bmatrix}$$

widerlegt. Hier gilt nämlich  $\text{per } A = \frac{3808}{13824} < \text{per}(AB) = \frac{3840}{13824}$ .

Noch eine weitere Vermutung ist geäußert worden, nämlich

$$\text{per}(AA^T) \leq \text{per } A.$$

Aber auch sie konnte widerlegt werden, und zwar von M. Newman durch das Gegenbeispiel

$$A = \frac{1}{2} \begin{bmatrix} 1 & 1 & 0 & 0 \\ 0 & 1 & 1 & 0 \\ 0 & 0 & 1 & 1 \\ 1 & 0 & 0 & 1 \end{bmatrix},$$

für welches  $\text{per } AA^T = \frac{9}{64} > \text{per } A = \frac{8}{64}$ .

Die van der Waerden'sche Vermutung hat auch noch für andere als doppelt stochastische Matrizen Sinn. Man betrachte z. B. die Klasse  $\mathfrak{M}(R, s)$  aller  $m \times n$ -Matrizen nichtnegativer Elemente mit vorgegebenem Vektor  $R = (r_i)$  bzw.  $S = (s_k)$  der Zeilen- bzw. Spaltensummen. Setzt man  $R = S = (1, \dots, 1)_n$ , so hat man wieder die Klasse der doppelt stochastischen Matrizen; hier ist wenigstens das Maximum der Permanentenfunktion bekannt; es ist nämlich gleich 1 und wird genau auf den Permutationsmatrizen angenommen.



Sei nun speziell  $m = n$  und

$$R = (1, n+1, \dots, n+1)$$

$$S = (n+1, \dots, n+1, 1).$$

Die Klasse  $\mathcal{W}(R, S)$  enthält z. B.

$$\begin{bmatrix} 1 & & & 0 \\ & \ddots & & \\ n & & \ddots & \\ & 0 & & \ddots \\ & & & & n & 1 \end{bmatrix}$$

Die Permanenten solcher Matrizen sind stets positiv, und es ist sinnvoll, nach Maximum und Minimum der Permanentenfunktion zu fragen.

Ist das Minimum von  $\text{per } A$  über diese Klasse = 1, wenn nur ganzzahlige Elemente zugelassen werden?

Eine scharfe Abschätzung nach oben ist seit kurzem bekannt (siehe [ 8 ] ):

Satz 6.3. Für  $A \in \mathcal{W}(R, S)$  mit  $R = (r_j)$ ,  $S = (s_j)$ ,

wobei o. B. d. A.  $r_1 \leq r_2 \leq \dots \leq r_n$ ,  $s_1 \leq s_2 \leq \dots \leq s_n$ , gilt

$$\text{per } A \leq \prod_{j=1}^n \min(r_j, s_j).$$

Angesichts der Schwierigkeiten dieser Probleme ist es sinnvoll, sich zunächst überhaupt auf die Klasse  $\mathcal{R}$  aller Null-Eins-Matrizen der Ordnung  $n$  mit Zeilen- und Spaltensummen  $= k$  ( $1 \leq k \leq n$ ) zu beschränken und die Extrema von  $\text{per}$  über  $\mathcal{R}$  zu bestimmen.

Hierzu gibt es zunächst eine untere Abschätzung von M. Hall:

Für  $A \in \mathcal{R}$  ist  $\text{per } A \geq k$  !

und für den allgemeineren Fall von Spaltensummen  $r_1, r_2, \dots, r_r$  eine Ungleichung von Mine

$$\text{per } A \leq \prod_{j=1}^n \frac{r_j + 1}{2}.$$

Darüber hinaus vermutete Mine

$$\text{per } A \leq \prod_{j=1}^n (r_j!)^{1/r_j}$$

und

$$\text{per } A \leq \prod_{j=1}^n (r_j!) \cdot \frac{1}{n!} \cdot \left( \frac{r_j + 1}{2} \right)^{\frac{n - r_j}{2}}.$$

Kombiniert man van der Waerden's Vermutung mit der ersten von Minc, so erhält man für  $A \in \mathfrak{R}$  offenbar die Abschätzung

$$k^n \cdot \frac{n!}{n} \leq \text{per } A \leq (k!) \cdot \frac{n}{k}.$$

Schließlich nennen wir noch die folgende Vermutung:

$$\left( \frac{n!}{n^n} \right)^r \cdot \prod_{j=1}^r (n+1-j)^n \leq L(r, n) \leq \prod_{j=1}^r (n+1-j)^{\frac{n}{n+1-j}},$$

wo  $L(r, n)$  die Anzahl der (nichtnormalisierten) lateinischen  $r \times n$  Rechtecke ist; dabei stützt sich die erste Ungleichung auf die van der Waerden'sche, die zweite auf die Minc'sche Vermutung.
